# Supplementary material for: Riemannian stochastic optimization methods avoid strict saddle points
Source: arXiv:2311.02374 source file (2023-11-04)
Supplement: Supplementary file 1 [file App-Prelim.tex]

%----------------------------------------------------------------------
%%% APP: APT
%----------------------------------------------------------------------
% !TEX root = ./Main.tex

We first focus on generalizing \cref{itm:sgd-critical} for min-max optimization. To proceed, recall first that critical points alone cannot capture the broad spectrum of algorithmic behaviors when \eqref{eq:MD} is not a gradient system:
already in \cref{fig:bilinear} we see a critical point surrounded by \emph{spurious} periodic orbits.
%\PM{This is an additional reason that I suggest following the (I) (II) structure, we get to familiarize the reader with the concept that ``set'' is more important than ``point'' in min-max problems.}
In addition, in dynamical systems many other spurious convergence phenomena are known, such as homoclinic loops, limit cycles, or chaos.
To account for this considerably richer landscape, we will need some definitions from the theory of dynamical systems.

\begin{definition}[\citealp{Ben99}]
\label{def:ICT}
Let $\set$ be a nonempty compact subset of $\points$.
%Let $\set\subseteq\points$ be nonempty and compact.
Then:
\begin{enumerate}
[\itshape a\upshape),leftmargin=.3in]
\item
%$\set$ is \emph{invariant} if $\flow[\ctime][\set] \subseteq \set$ for all $\ctime\geq0$.
$\set$ is \emph{invariant} if $\flow[\ctime][\set] = \set$ for all $\ctime\in\R$.
%\PM{Changed definition of ``invariant'' (and I'm avoiding the distinction with ``forward invariant'').}
\item \label{item:b}
$\set$ is \emph{attracting} if it is invariant and there exists a compact neighborhood $\cpt$ of $\set$ such that $\lim_{\ctime\to\infty} \dist(\flow,\set) = 0$ uniformly in $\point\in\cpt$.
\item
$\set$ is \acdef{ICT} if it is invariant and $\flowmap\vert_{\set}$ admits no proper attractors in $\set$.
\end{enumerate}
\end{definition}

\begin{remark*}
Equivalently, \ac{ICT} sets can be viewed as ``minimal connected periodic orbits up to arbitrarily small numerical errors'', \cf \citet[Prop.~5.3]{Ben99}.
The definition above is more convenient to work with because it provides the key insights in \cref{sec:RMsame?} below.
\end{remark*}

With all this preliminary work in hand, we are finally in a position to prove \crefrange{thm:avoid}{thm:attract}.

The heavy lifting for \cref{thm:ICT} is already provided by the fact that, under the requirements of \cref{thm:APT} and/or \cref{prop:APT}, $\curr$ is an \ac{APT} of the mean dynamics \eqref{eq:MD}, so it inherits its limit structure.
\cref{thm:avoid,thm:attract} on the other hand require a completely different set of techniques and involve a much finer analysis of the process in hand.
%borrowing from Conley's decomposition theorem (the so-called ``fundamental theorem of dynamical systems'').

\begin{proof}
%We consider two cases.
%First, if $\curr$ is unbounded, there is nothing to show.
%Otherwise, if $\curr$ is bounded, \cref{thm:ICT} shows that it is an \ac{APT} of the mean dynamics \eqref{eq:MD}.
By \cref{thm:APT}, $\curr$ generates \ac{APT} of the mean dynamics \eqref{eq:MD}.
Now, let $\limset = \intersect_{\ctime\geq\cstart} \cl(\apt{t,\infty})$ be the limit set of $\apt{\ctime}$, \ie the set of limit points of convergent sequences $\apt{\curr[\ctime]}$ with $\lim_{\run} \curr[\ctime] = \infty$.
Our claim then follows by the limit set theorem of \citet[Theorem 8.2]{BH96}.
\end{proof}

%As we discussed in the main part of our paper, the \ac{ICT} sets of $\minmax$ may exhibit a wide variety of structural properties (limit cycles, heteroclinic networks, etc.).
%As a complement to this, we show below that, in \emph{gradient} systems ($\vecfield = -\nabla\obj$ for some $\obj\from\points\to\R$), \ac{ICT} sets can only be compoments of equilibria.
%Specifically, building on a general result by \citet{Ben99}, we have:

\begin{proposition}
\label{prop:gradient}
Suppose that $\vecfield(\point) = -\nabla\obj(\point)$ for some $C^{\vdim}$-smooth potential function $\obj\from\points\to\R$ with a compact critical set $\crit(\obj) = \setdef{\sol}{\nabla\obj(\sol) = 0}$.
Then, every \ac{ICT} set $\set$ of \eqref{eq:MD} is contained in $\crit(\obj)$;
moreover, $\obj$ is constant on $\set$.
In particular, any \ac{ICT} set of \eqref{eq:MD} consists solely of critical points of $\obj$.
\end{proposition}

\begin{proof}
Under the stated conditions, the critical set $\sols \defeq \crit(\obj)$ of $\obj$ coincides with the set of rest points of \eqref{eq:MD}.
Moreover, by Sard's theorem \citep{Lee03}, $\obj(\sols)$ has zero Lebesgue measure and hence empty interior.
Our claim then follows from Proposition 6.4 of \citet{Ben99}.
\end{proof}
